# Supplementary material for: Proximate Tomonaga-Luttinger liquid in a spin-1/2 ferromagnetic XXZ chain compound
Source: arXiv:2411.06162 source file (2024-11-09)
Supplement: Supplementary file 1 [file Supplementary_R2.pdf]

## *Supplementary material*

### **Proximate Tomonaga-Luttinger liquid in a spin-1/2 ferromagnetic XXZ chain compound**

Boqiang Li,<sup>1,\*</sup> Xun Chen,<sup>1,\*</sup> Yuqian Zhao,<sup>1,\*</sup> Zhaohua Ma,<sup>1</sup> Zongtang Wan,<sup>1</sup> and Yuesheng Li<sup>1,†</sup>

<sup>1</sup>*Wuhan National High Magnetic Field Center and School of Physics,  
Huazhong University of Science and Technology, 430074 Wuhan, China*

We present here:

#### **I. Sample synthesis and characterization.**

Fig. S1. Powder x-ray diffraction and Rietveld refinement analysis.

Fig. S2. Image of as-grown single crystals.

Fig. S3. Electron spin resonance spectrum measured on the powder sample.

Table S1. Crystal structure refined from powder x-ray diffraction data.

Table S2. Crystal structure refined from single-crystal x-ray diffraction data.

#### **II. Numerical methods and models.**

Table S3. Density functional theory calculations.

Fig. S4. Validation of the effective XXZ model and finite-size effects.

Fig. S5. Negligible effects of weak antiferromagnetic next-nearest-neighbor intrachain coupling and validation of the stochastic series expansion method.

Fig. S6. Extraction of lattice specific heat for  $\text{LuCu}(\text{OH})_3\text{SO}_4$ .

Fig. S7. Determinating the strength of the interchain coupling.

Fig. S8. Phase diagram of  $\text{LuCu}(\text{OH})_3\text{SO}_4$ .

---

\* These authors contributed equally to this work

† [yuesheng\\_li@hust.edu.cn](mailto:yuesheng_li@hust.edu.cn)

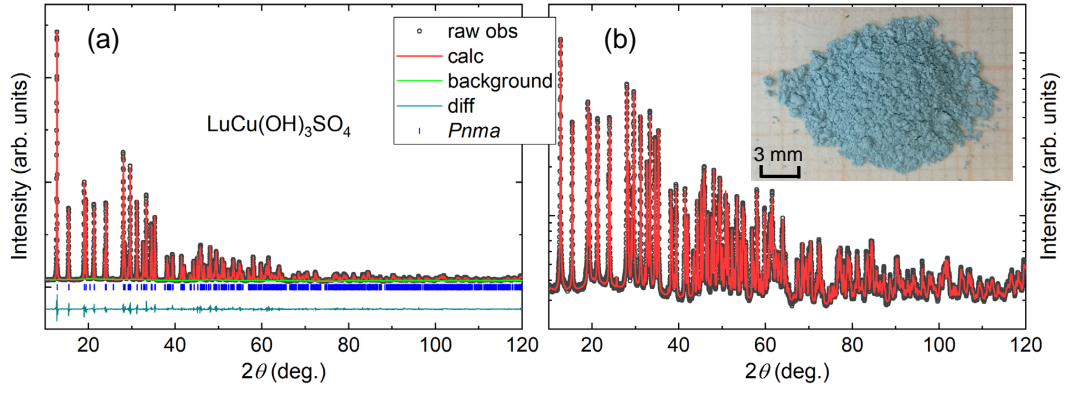

FIG. S1. (a) Powder x-ray diffraction and Rietveld refinement pattern for  $\text{LuCu}(\text{OH})_3\text{SO}_4$ . (b) A log10 intensity re-plot of the data. Inset: Powder sample ground from small crystals [see Fig. S2(a)].

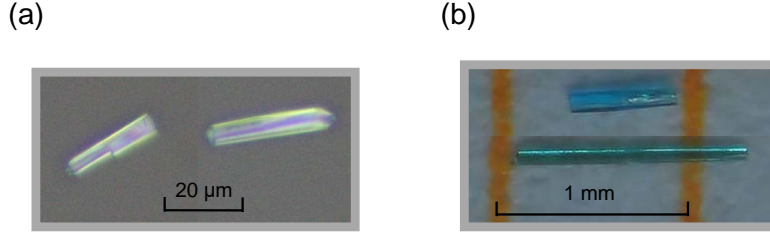

FIG. S2. Typical as-grown single crystals using a) CuO powders or b) copper plates as the Cu source in the synthesis processes. The  $b$  axis is along the longest dimension of each crystal. The slight color variations observed in samples may be attributed to differences in lighting and the microscopes used. The phase purities of  $\text{LuCu}(\text{OH})_3\text{SO}_4$  for both crystals shown in (b) have been confirmed through single-crystal XRD measurements. Both panels (a) and (b) are composed by stitching together two separate photographs, indicating that the images of the four crystals were captured under distinct lighting conditions. Furthermore, the photograph in (a) was acquired using a high-resolution optical microscope (Model: Zeiss Lattice SIM3) at a magnification of 1000 times, while (b) was captured using a standard microscope (Model: ZW-H3000) at a magnification of 50 times.

## I. SAMPLE SYNTHESIS AND CHARACTERIZATION

To synthesize  $\text{LuCu}(\text{OH})_3\text{SO}_4$ , we employed the traditional hydrothermal method, following the procedure reported in Ref. [1], and utilized CuO powder as the source of Cu,

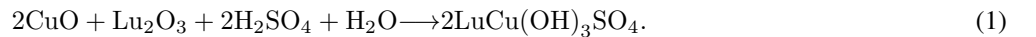

$\text{Lu}_2\text{O}_3$  ( $\geq 99.99\%$ , Adamas Reagent Co., Ltd, 1 mmol, 0.398 g), CuO ( $\geq 99\%$ , Adamas Reagent Co., Ltd, 2 mmol, 0.159 g), 1 M  $\text{H}_2\text{SO}_4$  (2 mmol, 2 mL), and 2 mL high-purity  $\text{H}_2\text{O}$  were mixed and charged into a 100 ml Teflon-lined autoclave. The sealed autoclave was heated to 503 K and maintained for 3 days. Light blue crystals were obtained after rinsing, filtration, and drying. The powder ground from the crystals was analyzed by x-ray diffraction (XRD), revealing no impurity phase (see Fig. S1). The refined crystal structure (Table S1) aligns well with the previously reported results [1]. The typical size of these crystals, measured by a microscope, is  $5 \times 30 \times 5 \mu\text{m}$  [see Fig. S2(a)], consistent with the previously reported work [1]. The electron spin resonance (ESR) spectrum measured on the powder indicates only about 0.45% quasi-free magnetic moments (Fig. S3). However, these crystals are too small for alignment, and larger-size single crystals are essential to collecting anisotropic magnetic data for  $\text{LuCu}(\text{OH})_3\text{SO}_4$ .

A log10 intensity re-plot of the powder XRD data is presented in Fig. S1(b). In Fig. S1(a), we also display the background (green line), which remains nearly constant. The powder sample utilized in this XRD measurement is ground from as-grown small crystals to prevent orientation preference. Each crystal encompasses  $\sim 4000 \times 50000 \times 8000 \times 4 \sim 6 \times 10^{12}$  spins ( $\gg 30^3 = 2700$  spins, see below), and therefore, any finite-size effects of crystals on magnetic properties should be negligible. The sizes of

TABLE S1. The crystal structure of  $\text{LuCu}(\text{OH})_3\text{SO}_4$  refined from the powder XRD data (Fig. S1). Please note that the positions and thermal parameters of H atoms weren't refined and were kept the same as in Ref. [1], as XRD is insensitive to H atoms. The occupancy fractions were set to "1" for all atoms, following the methodology in Ref. [1].

| space group               | <i>Pnma</i>                     |
|---------------------------|---------------------------------|
| <i>a</i>                  | 13.87629(7) Å                   |
| <i>b</i>                  | 6.07789(4) Å                    |
| <i>c</i>                  | 6.29356(3) Å                    |
| Cell volume, <i>Z</i> = 1 | 530.791(4) Å <sup>3</sup>       |
| Lu: <i>x, y, z</i>        | 0.41957(4), 0.25, 0.06358(8)    |
| <i>U</i> <sub>iso</sub>   | 0.0063(1)                       |
| Cu: <i>x, y, z</i>        | 0.5, 0, 0.5                     |
| <i>U</i> <sub>iso</sub>   | 0.0020(4)                       |
| S: <i>x, y, z</i>         | 0.3086(2), 0.75, 0.2704(4)      |
| <i>U</i> <sub>iso</sub>   | 0.0122(8)                       |
| O1: <i>x, y, z</i>        | 0.4152(3), 0.25, 0.4444(7)      |
| <i>U</i> <sub>iso</sub>   | 0.0004±0.0014                   |
| O2: <i>x, y, z</i>        | 0.4612(3), 0.9949(6), 0.7977(4) |
| <i>U</i> <sub>iso</sub>   | 0.022(2)                        |
| O3: <i>x, y, z</i>        | 0.2022(4), 0.75, 0.2974(7)      |
| <i>U</i> <sub>iso</sub>   | 0.013(2)                        |
| O4: <i>x, y, z</i>        | 0.3669(3), 0.75, 0.4676(8)      |
| <i>U</i> <sub>iso</sub>   | 0.0004±0.0016                   |
| O5: <i>x, y, z</i>        | 0.3251(3), 0.9402(6), 0.1414(5) |
| <i>U</i> <sub>iso</sub>   | 0.020(2)                        |
| H1: <i>x, y, z</i>        | 0.3680, 0.2500, 0.5000          |
| <i>U</i> <sub>iso</sub>   | 0.024                           |
| H2: <i>x, y, z</i>        | 0.4210, 0.9480, 0.7930          |
| <i>U</i> <sub>iso</sub>   | 0.024                           |
| <i>R</i> <sub>p</sub>     | 3.26%                           |
| <i>R</i> <sub>wp</sub>    | 4.50%                           |
| $\chi^2$                  | 10.31                           |

small crystals were analyzed using a high-resolution optical microscope [see Fig. S2(a)], and no scanning electron microscope (SEM) was employed. Additionally,  $\text{LuCu}(\text{OH})_3\text{SO}_4$  is a good insulator, rendering SEM measurements potentially unsuitable.

The powder x-ray diffraction exhibits sharp Bragg reflections (see Fig. S1), with a full width at half maximum of  $2\Delta\theta = 0.100^\circ$  at the strongest reflection  $2\theta = 12.71^\circ$ . By accounting for the instrument resolution of  $0.05^\circ$ , the intrinsic broadening  $2\Delta\theta_0$  is determined to be  $0.074^\circ$ . Using the Scherrer equation, the particle size of the ground powder (*P*) is estimated as  $P \geq \frac{K\lambda}{2\Delta\theta_0 \cos \theta} \sim 110$  nm, accounting for potential strain broadening. Here, *K* = 0.9 is the Scherrer constant, and  $\lambda = 0.154184$  nm is the x-ray wavelength. Each particle in the powder sample contains on average  $\sim \frac{2\pi P^3}{3V_0} \geq 5.3 \times 10^6$  spins ( $\gg 30^3 = 2700$  spins, see below), where  $V_0 = 0.53$  nm<sup>3</sup> is the cell volume (see Table S1), and each unit cell contains 4 spins.

To increase crystal size, we reduced the chemical reaction rate by using pure copper ( $\text{Cu} \geq 99.99\%$ ) plates as the Cu source,

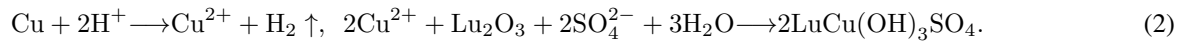

The corrosion process of copper plates by  $\text{H}_2\text{SO}_4$  is expected to be very slow, potentially allowing more time for crystal growth. The synthesis temperature of 503 K was maintained for 5 days and then cooled to room temperature at a rate of 8 K/hour. The typical size was increased to  $0.08 \times 1 \times 0.08$  mm, as shown in Fig. S2(b). Single-crystal XRD confirmed the  $\text{LuCu}(\text{OH})_3\text{SO}_4$  phase (Table S2) and indicated that the longest dimension of the crystal is along the *b* axis. We attempted various methods to optimize the synthesis, but the crystal size did not increase significantly further. Approximately 800 larger single crystals, with a total weight of  $\sim 10$  mg, grown using Eq. (2), were aligned along the *b* axis using GE varnish for magnetic property measurements. In sharp contrast, the aligned single-crystal sample exhibits no sharp ESR signals (see the main text), indicating the absence of quasi-free magnetic moments.

TABLE S2. The structural refinement of the single-crystal XRD data measured at 300 K. Positions and thermal parameters of H atoms were not refined and were kept consistent with Ref. [1]. Occupancy fractions were set to “1” for all atoms, following the methodology in Ref. [1].

|                                                                 |                                 |
|-----------------------------------------------------------------|---------------------------------|
| Size                                                            | 0.05×0.21×0.08 mm               |
| Molar mass                                                      | 385.6 g/mol                     |
| Space group                                                     | <i>Pnma</i>                     |
| <i>a</i>                                                        | 13.8541(5) Å                    |
| <i>b</i>                                                        | 6.0680(2) Å                     |
| <i>c</i>                                                        | 6.2865(2) Å                     |
| Cell volume, <i>Z</i> = 1                                       | 528.49(3) Å <sup>3</sup>        |
| Lu: <i>x, y, z</i>                                              | 0.41976(3), 0.25, 0.06365(6)    |
| <i>U</i> <sub>iso</sub>                                         | 0.0032(1)                       |
| Cu: <i>x, y, z</i>                                              | 0.5, 0, 0.5                     |
| <i>U</i> <sub>iso</sub>                                         | 0.0061(3)                       |
| S: <i>x, y, z</i>                                               | 0.3070(2), 0.75, 0.2671(4)      |
| <i>U</i> <sub>iso</sub>                                         | 0.0041(5)                       |
| O1: <i>x, y, z</i>                                              | 0.4175(5), 0.25, 0.433(1)       |
| <i>U</i> <sub>iso</sub>                                         | 0.006(2)                        |
| O2: <i>x, y, z</i>                                              | 0.4620(4), 0.9898(9), 0.8042(8) |
| <i>U</i> <sub>iso</sub>                                         | 0.006(1)                        |
| O3: <i>x, y, z</i>                                              | 0.2028(6), 0.75, 0.310(1)       |
| <i>U</i> <sub>iso</sub>                                         | 0.010(2)                        |
| O4: <i>x, y, z</i>                                              | 0.3629(6), 0.75, 0.466(1)       |
| <i>U</i> <sub>iso</sub>                                         | 0.011(2)                        |
| O5: <i>x, y, z</i>                                              | 0.3294(4), 0.947(1), 0.1405(9)  |
| <i>U</i> <sub>iso</sub>                                         | 0.016(1)                        |
| H1: <i>x, y, z</i>                                              | 0.3680, 0.2500, 0.5000          |
| <i>U</i> <sub>iso</sub>                                         | 0.024                           |
| H2: <i>x, y, z</i>                                              | 0.4210, 0.9480, 0.7930          |
| <i>U</i> <sub>iso</sub>                                         | 0.024                           |
| <i>h</i> range                                                  | −18 → 19                        |
| <i>k</i> range                                                  | −8 → 8                          |
| <i>l</i> range                                                  | −8 → 7                          |
| Reflections ( <i>I</i> > 0)                                     | 2484                            |
| Reflections ( <i>I</i> > 3σ( <i>I</i> ))                        | 2427                            |
| <i>R</i> ( <i>F</i> ) ( <i>I</i> > 3σ( <i>I</i> ))              | 3.7%                            |
| <i>R</i> <sub>w</sub> ( <i>F</i> ) ( <i>I</i> > 3σ( <i>I</i> )) | 4.5%                            |

## II. NUMERICAL METHODS AND MODELS

Nearest-neighbor Dzyaloshinsky-Moriya (DM) interaction is symmetrically allowed in LuCu(OH)<sub>3</sub>SO<sub>4</sub>. Through a standard symmetry analysis, we find that the nearly Heisenberg Hamiltonian invariant under the *Pnma* space group symmetry of LuCu(OH)<sub>3</sub>SO<sub>4</sub> is given as,

$$\mathcal{H}_{\text{DM}} + \mathcal{H}' = -J_1 \sum_j \mathbf{S}_j \cdot \mathbf{S}_{j+1} + D \sum_j (-1)^{j+1} (S_j^x S_{j+1}^y - S_j^y S_{j+1}^x) + \mathcal{H}', \quad (3)$$

where  $\mathcal{H}' = J_2 \sum_j \mathbf{S}_j \cdot \mathbf{S}_{j+2} + J_{\text{p1}} \sum_{\langle j, j_{\text{p1}} \rangle} \mathbf{S}_j \cdot \mathbf{S}_{j_{\text{p1}}} + J_{\text{p2}} \sum_{\langle j, j_{\text{p2}} \rangle} \mathbf{S}_j \cdot \mathbf{S}_{j_{\text{p2}}} + \dots$  represents interactions beyond the nearest neighbors, encompassing next-nearest-neighbor (NNN) intrachain coupling  $J_2$ , interchain exchanges  $J_{\text{p1}}$  and  $J_{\text{p2}}$ , and so forth. In our exact diagonalization (ED) and stochastic series expansion (SSE) simulations, we employ the periodic boundary condition  $\mathbf{S}_j \equiv \mathbf{S}_{j+N}$ , where  $N$  is an even number of spins considered.

To estimate the strengths of  $J_2$ ,  $J_{\text{p1}}$ , and  $J_{\text{p2}}$ , we conducted density functional theory (DFT) calculations with a typical

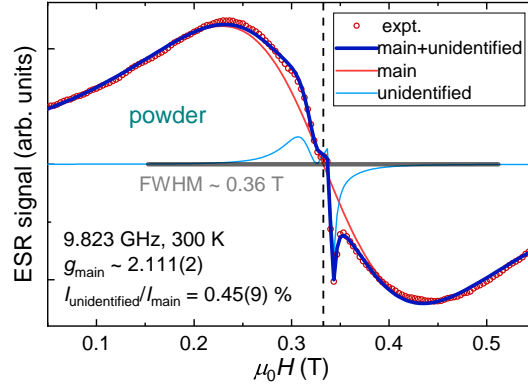

FIG. S3. Electron spin resonance (ESR) spectrum measured at 300 K on the powder sample ground from the smaller crystals [see Fig. S2(a)]. The observed sharp signals (unidentified) may originate from  $\sim 0.45\%$  of quasi-free- $\text{Cu}^{2+}$ -based impure phases. These sharp signals disappear in the ESR spectrum of the larger single crystals (see the main text).

TABLE S3. DFT calculations for exchange interaction energies using  $U = 5$  eV. The total and magnetic energies are relative values with respect to those of the fully ferromagnetic states, and the structural energy is independent of the magnetic structure.

| Supercell             | Positions of Cu                                                                                  | Magnetic structure                                     | Total energy | Magnetic energy      | Couplings          |
|-----------------------|--------------------------------------------------------------------------------------------------|--------------------------------------------------------|--------------|----------------------|--------------------|
| $1 \times 1 \times 1$ | (0,0,0)(0,0.5,0)<br>(0.5,0,0.5)(0.5,0.5,0.5)                                                     | $\uparrow\uparrow\uparrow\uparrow$                     | 0 K          | 0                    |                    |
|                       |                                                                                                  | $\uparrow\downarrow\uparrow\downarrow$                 | 100.7940 K   | $2J_1$               | $J_1 = 50.4$ K     |
|                       |                                                                                                  | $\uparrow\uparrow\downarrow\downarrow$                 | -0.2656 K    | $-4J_{p2}$           | $J_{p2} = 0.066$ K |
| $1 \times 2 \times 1$ | (0,0,0)(0,0.25,0)(0,0.5,0)(0,0.75,0)<br>(0.5,0,0.5)(0.5,0.25,0.5)<br>(0.5,0.5,0.5)(0.5,0.75,0.5) | $\uparrow\uparrow\uparrow\uparrow\uparrow\uparrow$     | 0 K          | 0                    |                    |
|                       |                                                                                                  | $\uparrow\downarrow\uparrow\uparrow\downarrow\uparrow$ | 98.8146 K    | $2J_1 - 4J_2$        | $J_2 = 0.49$ K     |
|                       |                                                                                                  |                                                        |              |                      |                    |
| $1 \times 1 \times 2$ | (0,0,0)(0,0.5,0)(0.5,0,0.25)<br>(0.5,0.5,0.25)(0,0,0.5)(0,0.5,0.5)<br>(0.5,0,0.75)(0.5,0.5,0.75) | $\uparrow\uparrow\uparrow\uparrow\uparrow\uparrow$     | 0 K          | 0                    |                    |
|                       |                                                                                                  | $\uparrow\uparrow\downarrow\downarrow\uparrow\uparrow$ | -9.9848 K    | $-4J_{p1} - 4J_{p2}$ | $J_{p1} = 2.4$ K   |
|                       |                                                                                                  |                                                        |              |                      |                    |

Coulomb repulsion of  $U = 5$  eV [7]. The DFT+ $U$  calculations were performed using the VIENNA AB INITIO SIMULATION PACKAGE (VASP) with the generalized gradient approximation [8–10]. We employed a  $4 \times 4 \times 4$  k-mesh, and residual forces were below  $0.003$  eV/Å in the fully optimized structure. The optimized structure remained unchanged in subsequent calculations of total energies for various magnetic structures and supercells. Electronic degrees of freedom relaxation were stopped when the total energy change and band structure energy change between two steps were both smaller than  $1 \times 10^{-7}$  eV = 1.2 mK. The precision was set to PREC = Accurate.

The strength of the nearest-neighbor exchange coupling monotonically decreases with increasing Coulomb repulsion  $U$ . DFT+ $U$  calculations suggest  $J_1 \sim 50$  K (see Table S3), roughly consistent with the experimental value obtained from the Curie-Weiss fits ( $J_1 \sim 65$  K). Therefore,  $U = 5$  eV is a suitable choice. Via DFT+ $U$  computations, we estimated  $J_2/J_1 \sim 1.0\%$ ,  $J_{p1}/J_1 \sim 4.8\%$ , and  $J_{p2}/J_1 \sim 0.1\%$ . The interactions beyond the nearest neighbors (terms in  $\mathcal{H}'$ ) are significantly smaller than the nearest-neighbor isotropic and DM couplings ( $J_1$  and  $D$  terms in  $\mathcal{H}_{\text{DM}}$ ).

We employed the SSE method within the general framework proposed in Refs. [11, 12]. To handle the antisymmetric DM interaction terms efficiently, we reduced the original DM model to the effective XXZ model through a unitary transformation (see the main text) [13]. While the transformation is mathematically strict, we carefully validated the reduced XXZ model by comparing it with finite-size ED calculations using the original DM model, as shown in Fig. S4. For chain lengths  $N$  less than  $\sim 30$ , ED/SSE simulations show evident finite-size effects at low temperatures of  $< 8$  K ( $\sim 0.1J_1$ ) despite the periodic boundary condition [see Fig. S4(b)], suggesting exotic ground-state properties of the spin-1/2 ferromagnetic XXZ chain system with long-distance unconventional entanglements. However, for  $N \geq 50$ , no finite-size effects are observed, and the 100-site ( $N = 100$ ) SSE calculations align well with integrable Bethe ansatz results at  $H \parallel z$  [see Figs. S4(b) and S5]. Therefore, we employed the 100-site SSE results for consistency throughout the main text. In practice, calculating the low-temperature specific heat exactly using the SSE method is challenging due to significant statistical errors [14]. The DFT+ $U$  calculations indicate a small strength for the NNN intrachain coupling, with  $J_2/J_1 \sim 1.0\%$  (see Table S3). Our many-body modeling further confirms the negligible

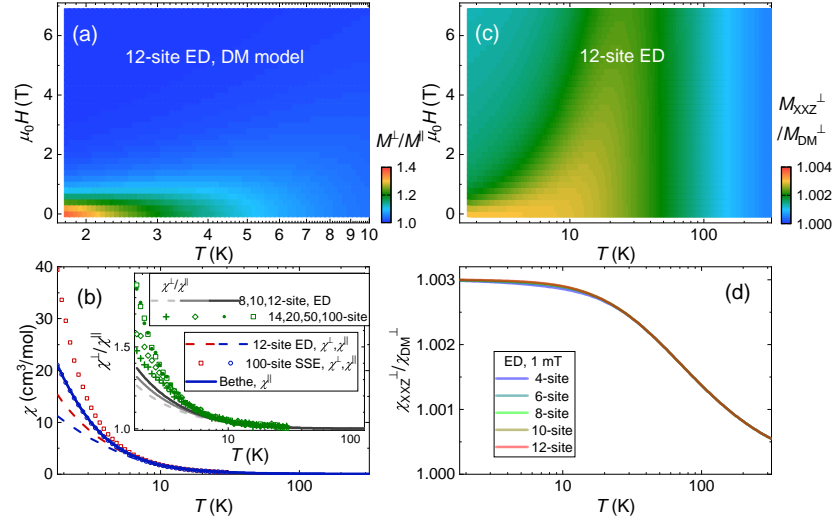

FIG. S4. Magnetization and susceptibilities calculated using ED, SSE, and Bethe ansatz methods, based on the DM and XXZ models,  $\mathcal{H}_{\text{DM}} = -J_1 \sum_j \mathbf{S}_j \cdot \mathbf{S}_{j+1} + D \sum_j (-1)^{j+1} (S_j^x S_{j+1}^y - S_j^y S_{j+1}^x)$  and  $\mathcal{H}_{\text{XXZ}} = -\sqrt{J_1^2 + D^2} \sum_j (S_j^x S_{j+1}^x + S_j^y S_{j+1}^y + \Delta S_j^z S_{j+1}^z)$ .  $J_1 = 65$  K and  $\Delta = 0.994$  (i.e.,  $D/J_1 = \sqrt{1/\Delta^2 - 1} = 0.11$ ) are used. (a) Anisotropy of magnetization ( $M^\perp/M^\parallel$ ) calculated using the 12-site ED method based on the DM model. “ $\perp$ ” and “ $\parallel$ ” represent the quantity with the magnetic field applied perpendicular and parallel to the  $z$  axis, respectively. (b) Calculated susceptibilities at  $\sim 0$  T ( $\chi^\perp$  and  $\chi^\parallel$ ). The inset shows  $\chi^\perp/\chi^\parallel$ . The DM model is used in the small-size ED calculations, whereas the XXZ model is used in the SSE and Bethe simulations. (c)  $M_{\text{XXZ}}^\perp/M_{\text{DM}}^\perp$ .  $M_{\text{XXZ}}^\perp$  and  $M_{\text{DM}}^\perp$  are 12-site ED calculated using the XXZ and DM models, respectively. (d)  $\chi_{\text{XXZ}}^\perp/\chi_{\text{DM}}^\perp$ .  $M_{\text{XXZ}}^\parallel \equiv M_{\text{DM}}^\parallel$  and  $\chi_{\text{XXZ}}^\parallel \equiv \chi_{\text{DM}}^\parallel$  are mathematically valid, and  $\chi_{\text{XXZ}}^\perp/\chi_{\text{DM}}^\perp$  ( $M_{\text{XXZ}}^\perp/M_{\text{DM}}^\perp$ ) is between 1 and 1.003, nearly independent of the chain length considered.

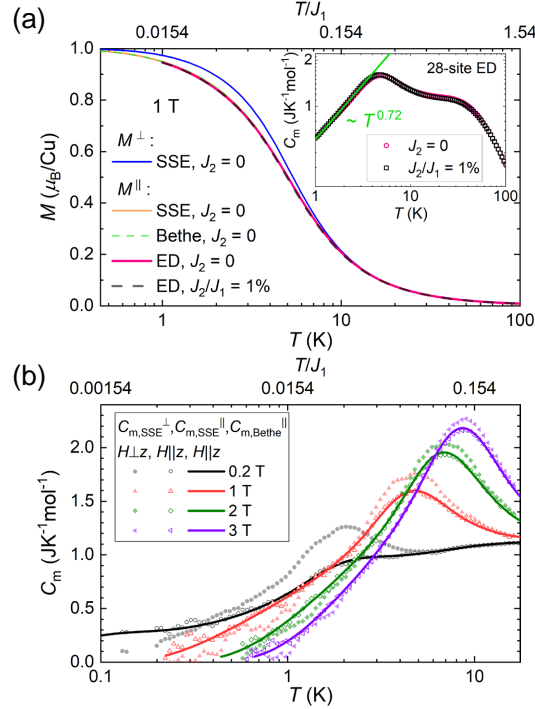

FIG. S5. (a) Magnetization calculated using the 100-site SSE, exact Bethe ansatz, and 28-site (Lanczos) ED [2] methods. The inset displays the ED specific heat, with the line showing the low- $T$  power-law behavior. The difference in quantities calculated with  $J_2 = 0$  and  $J_2/J_1 = 1\%$  is negligible, and finite-size effects are minimal for chain length  $N \geq 28$ . (b) Magnetic specific heat calculated using the 100-site SSE method, in comparison with the exact Bethe ansatz results. The Bethe method allows calculations only for quantities with the magnetic field applied parallel to the  $z$  axis [3–6]. The parameters  $J_1 = 65$  K and  $\Delta = 0.994$  are used.

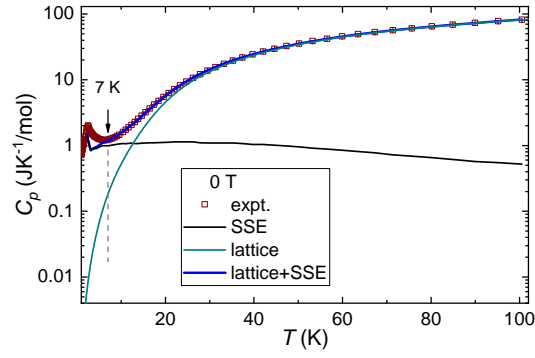

FIG. S6. Zero-field specific heat of  $\text{LuCu}(\text{OH})_3\text{SO}_4$ . The magnetic specific heat ( $C_{m,\text{SSE}}$ , black line) is calculated using the SSE method with the optimal parameter set I (see the main text). The blue line represents the fit to the experimental data (scatters) above 7 K, using the Debye-Einstein lattice function plus  $C_{m,\text{SSE}}$ .

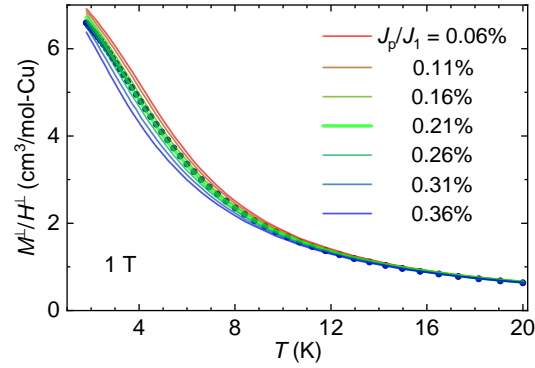

FIG. S7. Magnetization measured on the single-crystal sample with the magnetic field applied along the  $b$  axis ( $\mu_0 H^\perp = 1$  T). The colored lines show the SSE calculations with various  $J_p/J_1$  while keeping other parameters at their optimal values (see main text for details).

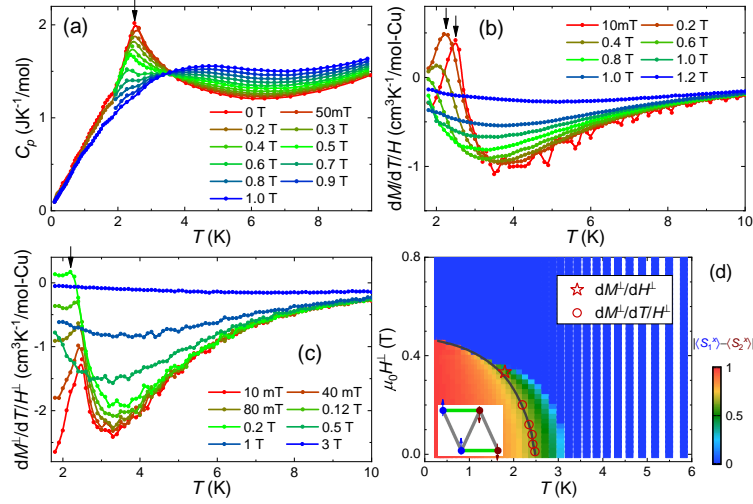

FIG. S8.  $B$ - $T$  phase diagram of  $\text{LuCu}(\text{OH})_3\text{SO}_4$ . (a) Specific heat measured on the powder sample at various applied fields. (b) The  $T$ -derivative magnetization ( $dM/dT/H$ ) measured on the powder sample at various applied fields. (c) The  $T$ -derivative magnetization ( $dM^\perp/dT/H^\perp$ ) measured on the single-crystal sample with magnetic fields applied along the  $b$  axis ( $H^\perp$ ). The arrows mark the critical temperatures  $T_c$ . (d) Interchain stripe-I order (lower inset) parameters calculated using the SSE method with a self-consistent mean-field treatment of interchain interactions (using the optimal parameters, as discussed in the main text). The critical field and temperatures obtained from the experimental  $dM^\perp/dH^\perp$  [see Fig. 4(b) in the main text] and  $dM^\perp/dT/H^\perp$  (see panel c) are displayed for comparison, and the thin line is a guide to the eyes.

impact of this  $J_2$  on both magnetization and specific heat, as illustrated in Fig. S5(a).

Using the optimal parameter set I, we calculated the SSE magnetic specific heat at 0 T,  $C_{m,SSE}$ , using a self-consistent mean-field treatment of interchain interactions (see the main text). Using  $C_{m,SSE} + C_{lattice}$ , we fitted the total specific heat of  $\text{LuCu}(\text{OH})_3\text{SO}_4$  measured at 0 T above  $\sim 7$  K (see Fig. S6). Here,  $C_{lattice}$  represents the lattice contribution of a standard Debye-Einstein function [2, 15], with the fitted parameters:  $\Theta_D = 97(1)$  K (wt. = 3),  $\Theta_{E1} = 133(1)$  K (wt. = 18),  $\Theta_{E2} = 283(3)$  K (wt. = 33), and  $\Theta_{E3} = 750(10)$  K (wt. = 102). Below  $\sim 7$  K,  $C_{lattice}$  becomes negligible compared to the magnetic specific heat  $C_m$ , with  $C_{lattice}/C_m < 0.1$  (see Fig. S6).

- 
- [1] H. J. Lu, K. Diefenbach, Z.-J. Li, H. L. Bao, X. F. Guo, J.-Q. Wang, T. E. Albrecht-Schmitt, and J. Lin, *Inorg. Chem.* **59**, 13398 (2020).
  - [2] J. Liu, L. Yuan, X. Li, B. Li, K. Zhao, H. Liao, and Y. Li, *Phys. Rev. B* **105**, 024418 (2022).
  - [3] M. Takahashi and M. Yamada, *J. Phys. Soc. Jpn.* **54**, 2808 (1985).
  - [4] P. Schlottmann, *Phys. Rev. Lett.* **54**, 2131 (1985).
  - [5] M. Takahashi, *World Sci.*, 299 (2001).
  - [6] M. Takahashi, *Czechoslov. J. Phys.* **53**, 1125 (2003).
  - [7] Y. Wang, S. Lany, J. Ghanbaja, Y. Fagot-Revurat, Y. P. Chen, F. Soldera, D. Horwat, F. Mücklich, and J. F. Pierson, *Phys. Rev. B* **94**, 245418 (2016).
  - [8] G. Kresse and J. Furthmüller, *Comp. Mater. Sci.* **6**, 15 (1996).
  - [9] G. Kresse and J. Furthmüller, *Phys. Rev. B* **54**, 11169 (1996).
  - [10] J. P. Perdew, K. Burke, and M. Ernzerhof, *Phys. Rev. Lett.* **77**, 3865 (1996).
  - [11] O. F. Syljuåsen and A. W. Sandvik, *Phys. Rev. E* **66**, 046701 (2002).
  - [12] A. W. Sandvik, *Phys. Rev. B* **59**, R14157 (1999).
  - [13] D. N. Aristov and S. V. Maleyev, *Phys. Rev. B* **62**, R751 (2000).
  - [14] A. W. Sandvik, *AIP Conf. Proc.* **1297**, 135 (2010).
  - [15] J. Liu, B. Liu, L. Yuan, B. Li, L. Xie, X. Chen, H. Zhang, D. Xu, W. Tong, J. Wang, and Y. Li, *New J. Phys.* **23**, 033040 (2021).
